# Supplementary material for: Optimizing Through Learned Errors for Accurate Sports Field Registration
Source: arXiv:1909.08034 source file (2020-05-28)
Supplement: Supplementary file 1 [file appendix.tex]

\cleardoublepage
\onecolumn
\appendix

\section{Supplementary appendix}

\subsection{Inference performance}
All the inference tasks were done on an Nvidia GTX 1080Ti GPU. To optimize a single frame, our framework can achieve 41.76 optimization iterations per second, thus 9.58 seconds per frame. The framework also supports batch inference. To optimize a batch with 64 frames, it can achieve 4.66 optimization iterations per second, thus in average 1.36 seconds per frame.
